# Supplementary material for: RedApt: An Adaptor for wav2vec 2 Encoding \\ Faster and Smaller Speech Translation without Quality Compromise
Source: arXiv:2210.08475 source file (2022-10-16)
Supplement: Supplementary file 1 [file supplementary.tex]

% This must be in the first 5 lines to tell arXiv to use pdfLaTeX, which is strongly recommended.
\pdfoutput=1
% In particular, the hyperref package requires pdfLaTeX in order to break URLs across lines.

\documentclass[11pt]{article}

% Remove the "review" option to generate the final version.
\usepackage[review]{emnlp2021}

% Standard package includes
\usepackage{times}

\usepackage{latexsym}

% For proper rendering and hyphenation of words containing Latin characters (including in bib files)
\usepackage[T1]{fontenc}
% For Vietnamese characters
% \usepackage[T5]{fontenc}
% See https://www.latex-project.org/hel][-09876`2][pohjgfdszaS,./?≥/documentation/encguide.pdf for other character sets

% This assumes your files are encoded as UTF8
\usepackage[utf8]{inputenc}

% This is not strictly necessary, and may be commented out,
% but it will improve the layout of the manuscript,
% and will typically save some space.
\usepackage{microtype}
\usepackage[normalem]{ulem}
\usepackage{booktabs}
\usepackage{threeparttable}

\usepackage{latexsym}
\usepackage{tabularx}
\usepackage{arydshln}

\usepackage{color,soul}
\definecolor{DarkBlue}{RGB}{28,81,140}
\definecolor{DarkRed}{RGB}{151,11,28}
\definecolor{DarkGreen}{RGB}{49,147,70}
\definecolor{LightGreen}{RGB}{129,234,108}
\makeatletter
  \newcommand\greenuline{\bgroup\markoverwith{\textcolor{green}{\rule[-0.7ex]{2pt}{0.4pt}}}\ULon}
  \UL@protected\def\redwave{\leavevmode \bgroup 
    \ifdim \ULdepth=\maxdimen \ULdepth 3.5\p@
    \else \advance\ULdepth2\p@ 
    \fi \markoverwith{\lower\ULdepth\hbox{\textcolor{red}{\sixly \char58}}}\ULon}
\makeatother

\usepackage{times}
\usepackage{multicol}
\usepackage{multirow}
\usepackage{graphicx}
\usepackage{graphicx} % for figures
\usepackage{tikz}
\usepackage{pgfplots}
\usepackage{booktabs}
\usepackage{microtype}
\usepackage{algorithm}
\usepackage{algorithmic}
\usepackage{amsbsy}
\usepackage{amsmath,soul}
\usepackage{soulpos}
\usepackage{amsmath}
\usepackage{multirow}
\usepackage{makecell}

\usepackage{amsmath,soul}
\usepackage{comment}
\usepackage{soulpos}
\usepackage{xcolor}
\usepackage[english]{babel}
\usepackage{blindtext}
\usepackage[shortcuts]{extdash}
\ulposdef{\ulnumaux}{%
   $\underset{\saveulnum}{\rule[-.7ex]{\ulwidth}{.4pt}}$}

\makeatletter
  \newcommand\greenuline{\bgroup\markoverwith{\textcolor{green}{\rule[-0.7ex]{2pt}{0.4pt}}}\ULon}
  \UL@protected\def\redwave{\leavevmode \bgroup 
    \ifdim \ULdepth=\maxdimen \ULdepth 3.5\p@
    \else \advance\ULdepth2\p@ 
    \fi \markoverwith{\lower\ULdepth\hbox{\textcolor{red}{\sixly \char58}}}\ULon}
\makeatother

%\aclfinalcopy % Uncomment this line for the final submission
%\def\aclpaperid{***} %  Enter the acl Paper ID here

%\setlength\titlebox{5cm}
% You can expand the titlebox if you need extra space
% to show all the authors. Please do not make the titlebox
% smaller than 5cm (the original size); we will check this
% in the camera-ready version and ask you to change it back.

% \title{Building and Learning Simultaneous Machine Translation from Professional Interpreters}
\title{Supplementary Material}
%Data Adaptation for SiMT via Style Transfer
% SiMT, Evaluation gap, Style Transfer, Pseudo interpretation, 
% Quantifying and Minimizing the Evaluation Gap of SiMT on Translation and Interpretation
% Bridging the Performance Gap between SiMT with Offline and Online Text via Style Transfer 
 
%\author{First Author \\
%  Affiliation / Address line 1 \\
%  Affiliation / Address line 2 \\
%  Affiliation / Address line 3 \\
%  \texttt{email@domain} \\\And
%  Second Author \\
%  Affiliation / Address line 1 \\
%  Affiliation / Address line 2 \\
%  Affiliation / Address line 3 \\
%  \texttt{email@domain} \\}

\date{}

\begin{document}
\maketitle

\bibliographystyle{acl_natbib}
\bibliography{custom}

%\appendix

\end{document}
