# Supplementary material for: RedApt: An Adaptor for wav2vec 2 Encoding \\ Faster and Smaller Speech Translation without Quality Compromise
Source: arXiv:2210.08475 source file (2022-10-16)
Supplement: Supplementary file 2 [file appendix.tex]

\section{Appendix}
\label{sec:appendix}
\mich{To be trimmed}
In this section, we will describe the process of collecting genuine data and creating a dataset, mirroring the real-life scenarios. We then present a test set which is annotated by bilingual annotators, thus ensuring the genuineness of our experimental results and analysis. 

\subsection{Corpus Collection}


\begin{comment}
\begin{figure}
    \centering
    \includegraphics[width=7cm]{ASR.pdf}
    \caption{The transcription in SRC and transcription in TRG is a suitable parallel corpus to build simultaneous interpration system.}
    \label{fig:my_label}
\end{figure}
\end{comment}

To test our hypothesis, we decided to collect genuine data from European Parliament (EP) Plenary where debates are carried out among representatives of member states of the European Union who speak their native languages, and thus to facilitate communication, simultaneous translation services are provided on site. From 2008/09/01 to 2012/11/22, transcriptions of speeches and corresponding post-edited translations are available for each language spoken, and audios of interpreting can be found next to a particular speaker's profile. We selected German-English as our target language pair. To pick out the target language, we used a number of heuristics methods to identify the nationality of the speakers and crawled the three sources of data for this period accordingly. Out of the sources, transcriptions of the speeches (in German) and automatic speech recognition (ASR) outputs of the audios (in English), creation of which will be described later, are aligned as training data in this work. Post-edited translations are used to aid the pairing process. Note post-edited translations are only available during this period due the changes of EP's policies, while audios and transcriptions are provided from 2004 till today. We will leave collecting and making use of the full data in our future work. As a results, we downloaded 238 debates and 2415 audio files in the mp4 format, with a total size of 500GB. We then used google speech API to transcribe and normalize ASR outputs and thus 19368.24 minutes were transcribed. We also used posted-edited translations to maintain name entities. This process yielded 10,481 dialogues (bitexts).

%with a total cost of 697.257 USD.




%For each debate on particular day, there are multiple speakers talking in their native language $f$. europarl provides a selection of viewer languages of language $e$ which employs sets of professional interpreter $I$ that translates $f$ into $e$. The interpreter is not working when $f=e$. europarl also provides a post-edited version of each speaker dialogues in languages $e$.

\begin{comment}
\begin{table}[h!]
\small
    \centering
    \begin{tabular}{c|c|c|c}
        Orig speech & Viewer Lang & Interp Speech & PE Trans\\ \hline
        $x$ & $f$ & $x$ & $\hat{x}$   \\
        $x$ & $e$ & $y$ & $\hat{y}$   \\
    \end{tabular}
    \caption{Here x is the speech in native language $f$ and y is the interpretation in language $e$ which satisfies $y=I(x)$. The post-edited translation is the $\hat{x}$ and $\hat{y}$.}
    \label{tab:my_label}
\end{table}
\end{comment}



\subsection{Parallel Dataset Creation}

%When dealing with crawled corpus, researchers commonly apply techniques such as arbitrary sequence truncation \cite{sperber2018kit}, removal of wrong language code and long sequences \cite{matusov2018neural}. 

To build a dataset with high-quality, we enacted a series of sophisticated automatic and manual pre-processing steps to clean and filter dialogues.  The total number of dialogues is 5,239. Initially, we removed 1,183 dialogues whose source was non-German, as debates were carried out among the representations of the member states of EU and only German was needed for this study. To keep the essence of the debates, we filtered out below non-essential components and considered them as transitions between conversations: i) dialogues with less than 20 tokens; ii) dialogues which have pre-defined signals (e.g., "the vote will take place") if they have less than 100-150 words, depending on the signals. The number of data points removed is 2,174. Human investigation on disregarded dialogues confirmed these heuristics. We also disgarded those whose source and translation have different number of sentences, which was, however, rare. The above steps yielded of a number of 1,872 data points. Following that, we manually deleted dialogues which were non-essential contents of the debates. Meanwhile, we truncated transcripts whose first and last sentences did not match the corresponding post-edited translation; most of deleted sentences were results of imperfect audio segmentation. After the manual process, 987 dialogues are retained, representing the essence of the debates. 


The procedure for obtaining parallel translation pairs is described as follows. Firstly, we align sentences in the post-edited translation with those in the transcript of live interpretation, both of which were in English. As the transcript may not be well segmented during the automatic speech recognization process, we identified sentences in the transcript with stanza\footnote{\url{https:/ /github.com/stanfordnlp/stanza}} \cite{qi2020stanza}. Note each source sentence and post-edited translation sentence in the collected dialogues may consist of several sentences. We call them super-sentences and we don't perform sentence splitting on those super-sentences yet. Next, for each dialogue, we segmented the English transcript sentences based on the number of super-sentences in the corresponding translation using dynamic programming, details of which will be discussed in the following section. This step is important due to the fact that unlike post-edited translations which tend to be long and formal, in real-life SI scenarios a source sentence (i.e., German in our case) can often broken into multiple smaller pieces. Hence, it is necessary to recognize and rejoin those pieces into chunks. We chose the candidate, i.e., segmented sentences in the live English transcript, which had the highest similarity score to the English translation in the semantic space\footnote{Similarity scores are calculated with \url{https://github.com/UKPLab/sentence-transformers/tree/master/sentence_transformers}}, as the output. More specifically, each of the chunks was semantically similar to one super-sentence in the translation. Since such a super-sentence in any dialogue corresponds to a long, formal German super-sentence, equally each of the chunks can be allocated to that source sentence. This gives us a super-sentence-level dataset in our work, consisting of 3,683 data points. This step is implemented on English pairs, as we believe calculating similarity scores in the same language yields more accurate results than comparing the semantic similarity between different languages.

Following that, we also tried to segment super-sentences with almost the identical procedure\footnote{The only difference here is that we used a multilingual encoder}. However, after inspecting the outputs of the resulting dataset, we noticed it had a large variations of noises in the sentence-level translation pairs. The noised pairs are contributed by many factors, such as imprecise similarity scores and incorrect punctuation insertion in the process of normalizing ASR outpus. Hence, we decided to recruit a bilingual German-English speaker to pair sentences manually to create translation pairs that genuinely occur in SI, and they become the test data in this work. We will describe the details of the annotation process in the following section.

%In the second stage, further alignment needs to be done between each ``single" German sentence and the allocated English chucks. As described earlier, this is based on the observation that a source sentence may contain more than one sentence; thus, to construct sentence-level translation pairs, it needs to be separated beforehand. After that, for each segmented source sentence, we find the best candidate from the target English chuck in the similar manner as stage one\footnote{Similarity scores are calculated with a multi-lingual encoder \url{https://github.com/yannvgn/laserembeddings}}. 
%For fair comparison with above source-transcript pairs, our last stage is to construct translation pairs out of sources and translations and this is performed similarly the second stage. 
%Stages 2 and 3 yield a total number of 10,561 instances. 
%We finally create our second sentence-level dataset, which has 10,501 data instances. Note that above methodology can be applied to other languages in any future work in SI.


\subsection{Sequence Segmentation/Alignment with Dynamic Programming}
In \cite{lison2016opensubtitles2016}, sentence segmentation is mainly dependant on occurrences of sentence-ending markers, and alignment heavily rely on timing information, whereas in \cite{cettolo2012wit3} sentence alignment is dependant on heuristic checks. These are not applicable to our crawled data in which outputs are in the normalized ASR format which inherently exhibit noises and no timing stamps are available. Instead, we use a dynamic programming algorithm, as shown in Algorithm \ref{alg:npi}, to segment target utterances and perform alignment in the semantic space. As can be seen from \ref{tab:example}, each source sentence has its own correspondence of translation, so we only need to align segments of sentences in transcripts to that translation sentence, in order to have a parallel source-transcript corpus. Hence, we dynamically divide transcript sentences by the number of translation sentences, calculate the similarity score for each pair while considering the accumulated scores for sequences preceding it. We then traceback the candidate with the best score. The time complexity of this algorithm is $O(KN^2)$, where $K$ is the number of source sentences and $N$ is the number of target utterance. This algorithm is applicable to creating both the chuck-level and sentence-level parallel datasets.

\input{algorithms/alg-dp}
%\input{tables/example_dialogues}

\subsection{Test Set Annotation}
To build the annotated test set, we firstly randomly sampled 400 pairs from the super-sentence-level dataset and split super-sentences into sentence-level. Then we asked the annotator to match the correct target sentence(s) against each source sentence. Specifically, we instructed the annotator to find the English texts for each German sentence and in the extreme case of impossible aligning to one German sentence, multiple sentences are allowed. In addition to that, to comply with human speaking styles and , We allowed the following phenomena: 1) the minor omission of unimportant English texts as long as the main idea of German text is conveyed (such as conjunctions), as it is in real-life SI situations; 2) repeated words in transcripts as it does happen with interpreting or when anyone speaks. It took 38-hour for our annotator to finish the job. We cross checked the resulting pairs to enforce quality control. Having this data set is crucial in our work, as our goal is to investigate how the State-of-the-Art MT models behave on the real-life data, not on the datasets which mirror SI scenarios. Yet since human annotation is time-consuming and expensive, this process is not scalable to the whole dataset. 
\mich{Michelle: I wasn't sure if it was right not to edit the English transcripts. The reasons I didn't ask the annotator to edit, though, were 1) it's expensive; 2) it's hard to do so, as it requires to correct errors that occurred when converting audio to texts. For example, the sound "parliament" may be transcripted to "apartment", and the annotator has to think hard to tell they are actually the same thing.}
